# Supplementary material for: Curvature in graphene nanoribbons generates temporally and spatially focused electric currents
Source: arXiv:1501.06934 ancillary file (2015-01-27)
Supplement: Supplementary file 1 [file gnr_curved_SI_final.compressed.pdf]

# Supplemental Information:
# Curvature in graphene nanoribbons generates temporally and spatially focused electric currents

C. G. Rocha,[1,2] R. Tuovinen,[1] R. van Leeuwen,[1] and P. Koskinen[1]

[1]*Nanoscience Center, Department of Physics, University of Jyväskylä, 40014 Jyväskylä, Finland*
[2]*School of Physics, Trinity College Dublin, Dublin 2, Dublin, Ireland*

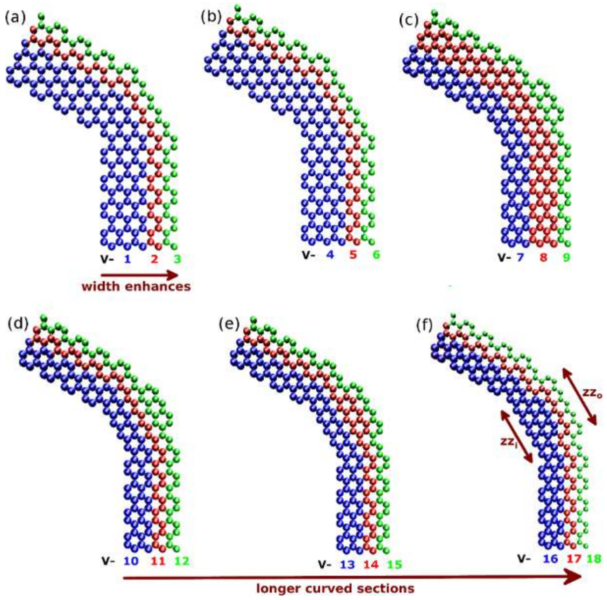


FIG. 1: (Color online) Systematic set of curved graphene nanoribbon (CGNR) samples with 60° angles. There are three different widths (blue thinnest, red intermediate, and green widest) for each type of curvature. Notation for each sample is given at the bottom of each panel: (a) V-1, V-2, V-3; (b) V-4, V-5, V-6; (c) V-7, V-8, V-9; (d) V-10, V-11, V-12; (e) V-13, V-14, V-15; (f) V-16, V-17, V-18. Their structural information, including the number of zigzag segments at the inner (zz$_i$) and outer (zz$_o$) edges, are shown in Table I. All samples are hydrogen-terminated, but hydrogens are omitted from the figures for clarity. The samples discussed in the main text are V-1 (sample V$_\mathrm{a}$) and V-18 (sample V$_\mathrm{b}$).

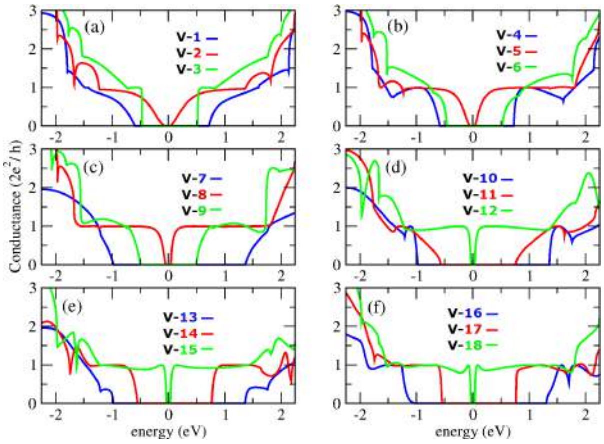


FIG. 2: (Color online) Conductance as a function of energy for all CGNRs of Fig. 1 (using corresponding ordering).

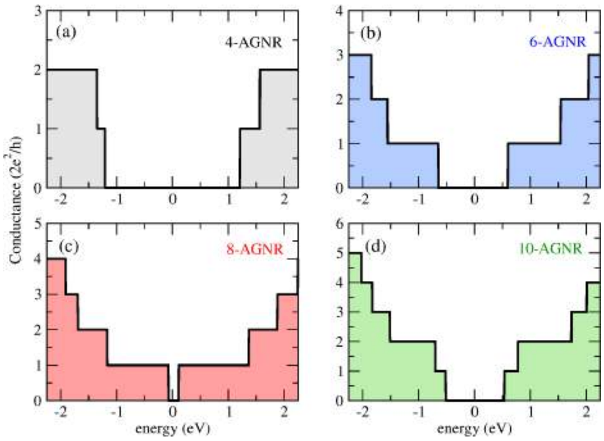


FIG. 3: (Color online) Conductance as a function of energy for straight armchair graphene nanoribbons of width $N$ =4, 6, 8, 10.

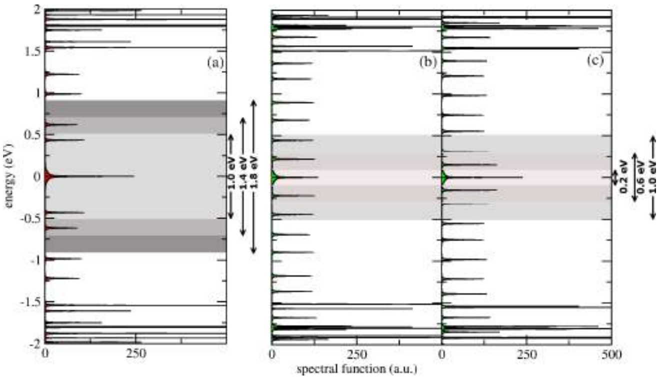


FIG. 4: (Color online) Spectral function for the (a) V-2 (sample $V_a$ in main text), (b) V-9, and (c) V-18 (sample $V_b$ in main text) CGNRs. Fermi energy is at 0 eV. Gray areas span the relevant energy ranges at different biases, to better identify the possible states involved in transitions.

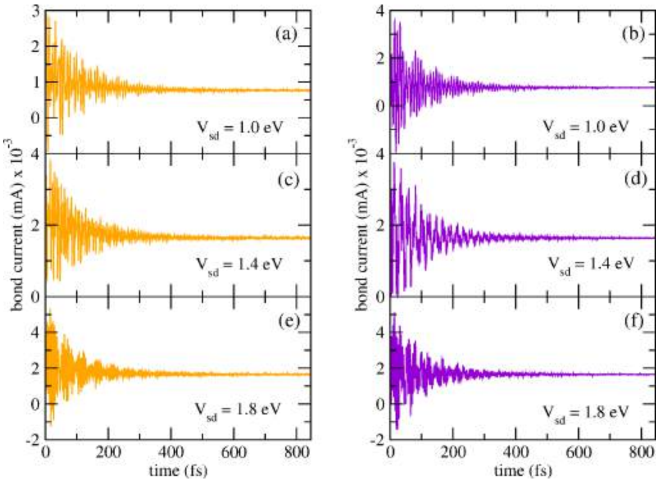


FIG. 5: (color online) Long-time currents through V-2 CGNR (sample $V_a$ in main text) at bridge B1 (left panels) and at bridge B2 (right panels), using bias voltages $V_{SD}$ = 1.0, 1.4, and 1.8 eV (top to bottom panels).

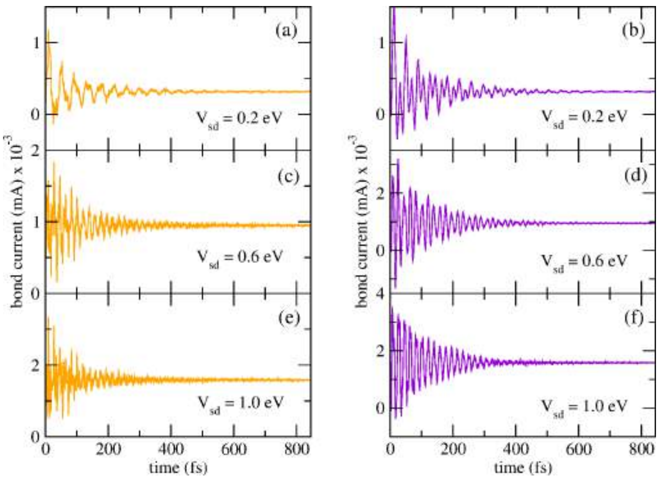


FIG. 6: (color online) Long-time currents through V-9 CGNR at bridge B1 (left panels) and at bridge B2 (right panels), using bias voltages $V_{\mathrm{SD}} = 0.2$, 0.6, and 1.0 eV (top to bottom panels).

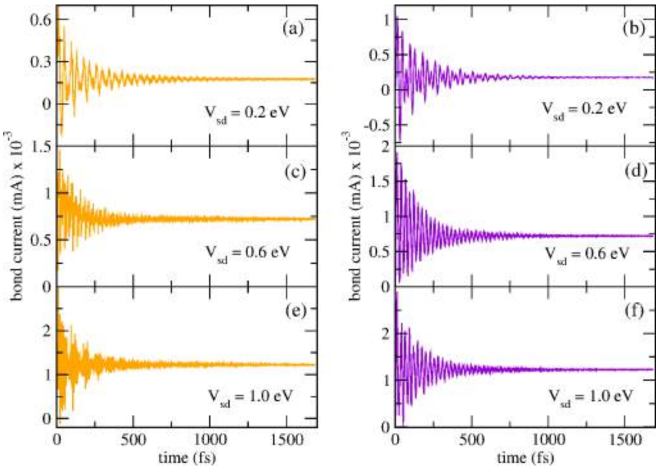


FIG. 7: (color online) Long-time currents through the V-18 CGNR (sample $V_b$ in main text) at bridge B1 (left panels) and at bridge B2 (right panels), using bias voltages $V_{\mathrm{SD}} = 0.2$, 0.6, and 1.0 eV (top to bottom panels).

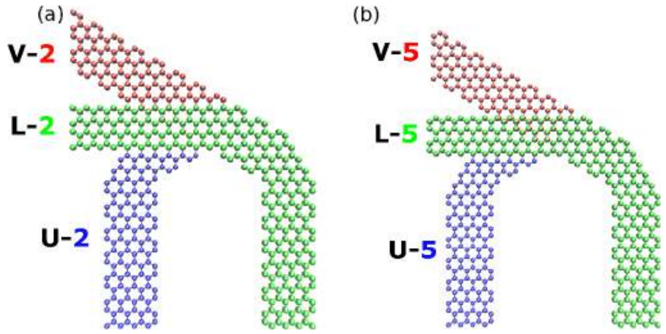


FIG. 8: (Color online) Set of CGNR samples with 90° (green) and 180° (blue) angles, in addition to the familiar 60° (red) angle. (a) CGNRs V-2 (sample $V_a$ in main text), U-2 (sample U in main text), and L-2 (sample L in main text) have short curved parts. (b) CGNRs V-5, U-5, and L-5 have longer curved parts. All samples are hydrogen-passivated, but the hydrogens are omitted from the figure for clarity.

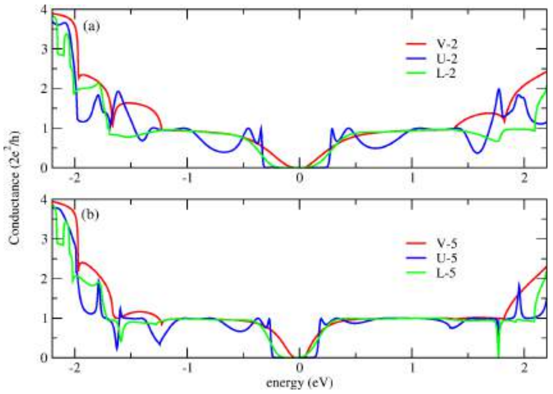


FIG. 9: (Color online) Conductance as a function of energy for the CGNRs shown in Fig. 8.

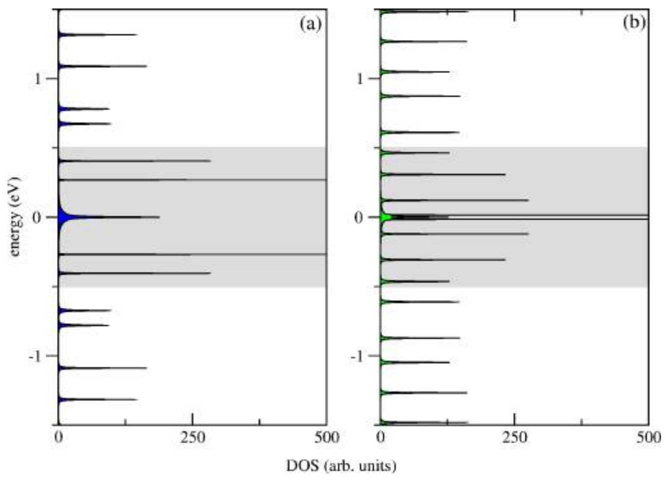


FIG. 10: (Color online) Spectral function for the (a) U-2 (sample U in main text) and (b) L-2 (sample L in main text) CGNRs. Fermi energy is at 0 eV. Gray areas span the relevant energy ranges at different biases, to better identify the possible states involved in transitions.

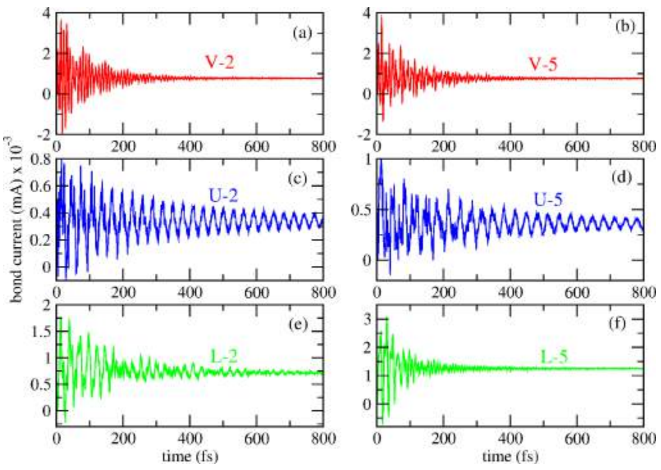


FIG. 11: (color online) Long-time currents through the CGNRs (a) V-2, (b) V-5, (c) U-2, (d) U-5, (e) L-2, and (f) L-5 at bias $V_{\mathrm{SD}} = 1.0$ eV. Currents are measured at bridges in the middle of the curved section.

TABLE I: Structural parameters of the V-junctions shown in Fig. 1: number of zigzag segments in the inner ($zz_i$) and outer ($zz_o$) edges, number of armchair segments located in the outer curved edge (ac), lead type (GNR) and its width (W), inner ($R_i$) and outer ($R_o$) mean radius of curvature, and the mean width of the curved part ($W_c = R_o - R_i$).

| **V-junctions** | | | | | | | | |
|---|---|---|---|---|---|---|---|---|
| **Label** | $zz_i$ | $zz_o$ | ac | GNR | W (Å) | $R_i$ (Å) | $R_o$ (Å) | $W_c$ (Å) |
| V-1 | 0 | 4 | 0 | 6-AGNR | 6.12 | 11.80 | 16.20 | 4.40 |
| V-2 | 0 | 6 | 0 | 8-AGNR | 8.57 | 11.80 | 18.40 | 6.60 |
| V-3 | 0 | 8 | 0 | 10-AGNR | 11.02 | 11.80 | 20.62 | 8.82 |
| V-4 | 2 | 6 | 0 | 6-AGNR | 6.12 | 14.01 | 18.40 | 4.39 |
| V-5 | 2 | 8 | 0 | 8-AGNR | 8.57 | 14.01 | 20.62 | 6.61 |
| V-6 | 2 | 10 | 0 | 10-AGNR | 11.02 | 14.01 | 22.84 | 8.83 |
| V-7 | 4 | 6 | 0 | 4-AGNR | 3.67 | 16.02 | 18.41 | 2.39 |
| V-8 | 4 | 10 | 0 | 8-AGNR | 8.57 | 16.02 | 22.84 | 6.82 |
| V-9 | 4 | 8 | 2 | 10-AGNR | 11.02 | 16.02 | 25.95 | 9.93 |
| V-10 | 6 | 8 | 0 | 4-AGNR | 3.67 | 18.42 | 20.62 | 2.20 |
| V-11 | 6 | 10 | 0 | 6-AGNR | 6.12 | 18.42 | 22.84 | 4.42 |
| V-12 | 6 | 8 | 2 | 8-AGNR | 8.57 | 18.42 | 25.90 | 7.48 |
| V-13 | 8 | 10 | 0 | 4-AGNR | 3.67 | 20.64 | 22.84 | 2.20 |
| V-14 | 8 | 8 | 2 | 6-AGNR | 6.12 | 20.64 | 25.91 | 5.27 |
| V-15 | 8 | 10 | 2 | 8-AGNR | 8.57 | 20.64 | 28.27 | 7.63 |
| V-16 | 10 | 8 | 2 | 4-AGNR | 3.67 | 22.65 | 25.86 | 3.21 |
| V-17 | 10 | 10 | 2 | 6-AGNR | 6.12 | 22.65 | 28.23 | 5.58 |
| V-18 | 10 | 12 | 2 | 8-AGNR | 8.57 | 22.65 | 30.57 | 7.92 |
